# Supplementary material for: Adaptive Periodic Averaging: A Practical Approach to Reducing Communication in Distributed Learning
Source: arXiv:2007.06134 source file (2021-01-19)
Supplement: Supplementary file 1 [file appendix.tex]

\section{Artifact Description}

%%%%%%%%%%%%%%%%%%%%%%%%%%%%%%%%%%%%%%%%%%%%%%%%%%%%%%%%%%%%%%%%%%%%%
\subsection{Abstract}
The artifact includes all of the programs that are needed to reproduce the evaluation results in the paper. 
The programs should be executed on an HPC cluster with at least 16 GPU nodes. 
To reproduce the execution time and the communiation time reported in the paper, the GPUs need to be Nvidia Tesla P100, and the computing nodes need to be connected by 100 Gbps InfiniBand. 
The artifact will print out the training loss and the test error for each epoch of the training process.  
The artifact will also print out the total computation time and communication time for each training task. 

%%%%%%%%%%%%%%%%%%%%%%%%%%%%%%%%%%%%%%%%%%%%%%%%%%%%%%%%%%%%%%%%%%%%%
\subsection{Description}

\subsubsection{Check-list (artifact meta information)}

{\small
\begin{itemize}
  \item {\bf Program:} (1) original full communication SGD, (2) constant periodic parameter averaging SGD, (3) quantized gradient SGD, (4) adaptive periodic averaging SGD
  \item {\bf Data set:} (1) CIFAR10, (2) ILSVRC2012 ImageNet
  \item {\bf Output:} program results including training loss, test error, computation time, and communication time. 
  \item {\bf Experiment workflow:} a bash script is provided in each directory to automatically start the execution
\end{itemize}
}

\subsubsection{How software can be obtained (if available)}
The artifact is publicly available at "the pointer will be provided if the paper is accepted". 
The  programs are about 12KB. 

\subsubsection{Hardware dependencies}
An HPC cluster with 16 computing nodes each equipped with an Nvidia Tesla P100 GPU is needed. 

\subsubsection{Software dependencies}
CUDA9.2, NCCL2.3.7, PyTorch1.0.0

\subsubsection{Datasets}
The CIFAR10 and ImageNet datasets are available online. 
CIFAR10 is download automatically in the PyTorch training code. 
We provide a 'get\_imagenet.sh' script in the top directory. It will automatically download and prepare the ImageNet dataset. Imagenet takes about 150GB disk space. 
%%%%%%%%%%%%%%%%%%%%%%%%%%%%%%%%%%%%%%%%%%%%%%%%%%%%%%%%%%%%%%%%%%%%

%%%%%%%%%%%%%%%%%%%%%%%%%%%%%%%%%%%%%%%%%%%%%%%%%%%%%%%%%%%%%%%%%%%%%
\subsection{Experiment workflow}

There are three steps to conduct the experiments:

1) Download the datasets: This can be done by executing the 'get\_imagenet.sh' script in the top directory. 

2) Execute the codes: Each directory contains the four different versions of SGD for a specific neural network model.  
The programs can be directly executed as python scripts. 
A 'run.sh' script is also provided in each directory for running the four versions of SGD one-by-one automatically. 
Another 'run\_trickle.sh' script is provide for throttling the connection bandwidth to 10Gbps and executing the programs with the emulated 10Gbps connection. 

3) Collect results: a python script 'plot.py' is provided in each directory that collects the output of execution, and plots the training loss, test accuracy and execution time as in Fig. 4, 5, 6, 7. 

%%%%%%%%%%%%%%%%%%%%%%%%%%%%%%%%%%%%%%%%%%%%%%%%%%%%%%%%%%%%%%%%%%%%%
\subsection{Evaluation and expected result}
The plots should be very close to Fig. 4, 5, 6, 7 in the paper.
